# Supplementary material for: $\mathcal{CP}$-violation sensitivity of closed-shell radium-containing polyatomic molecular ions
Source: arXiv:2312.11687 source file (2023-12-20)
Supplement: Supplementary file 1 [file supplement.pdf]

# Supplementary material of “ $\mathcal{CP}$ -violation sensitivity of closed-shell radium-containing polyatomic molecular ions”

Konstantin Gaul,<sup>1,\*</sup> Nicholas R. Hutzler,<sup>2</sup> Phelan Yu,<sup>2</sup> Andrew M. Jayich,<sup>3</sup> Miroslav Iliaš,<sup>4</sup> and Anastasia Borschevsky<sup>5</sup>

<sup>1</sup>*Fachbereich Chemie, Philipps-Universität Marburg, Hans-Meerwein-Straße 4, 35032 Marburg*

<sup>2</sup>*California Institute of Technology, Pasadena, CA 91125, USA*

<sup>3</sup>*Department of Physics, University of California, Santa Barbara, California 93106, USA*

<sup>4</sup>*Department of Chemistry, Faculty of Natural Sciences, Matej Bel University, Tajovského 40, 97401 Banská Bystrica, Slovakia*

<sup>5</sup>*Van Swinderen Institute for Particle Physics and Gravity, University of Groningen, 9747 AG Groningen, The Netherlands*

(Dated: December 20, 2023)

Table I. Electronic structure enhancement factors of  $\mathcal{P}$ ,  $\mathcal{T}$ -violation in Ra-containing closed-shell molecular ions computed at the level of DCHF/dyall.cv3z+sp(d) and DCKS/dyall.cv3z+sp(d) employing various exchange correlation functionals.

| Molecule                        | Functional | $W_d^m / \frac{10^{20} \text{ Hz h}}{e \text{ cm}}$ | $W_s^m / (h \text{ Hz})$ | $W_T / (h \text{ kHz})$ | $W_P / (h \text{ Hz})$ | $W_m / \frac{10^{17} \text{ Hz h}}{e \text{ cm}}$ | $W_S / \frac{\text{MHz h}}{e \text{ fm}^3}$ |
|---------------------------------|------------|-----------------------------------------------------|--------------------------|-------------------------|------------------------|---------------------------------------------------|---------------------------------------------|
| RaSH <sup>+</sup>               | HF         | 36.0                                                | 93.1                     | −4.39                   | −17.2                  | −1.90                                             | −2.19                                       |
|                                 | BHandH     | 31.9                                                | 82.9                     | −3.91                   | −15.3                  | −1.68                                             | −1.95                                       |
|                                 | PBE0       | 30.0                                                | 78.2                     | −3.70                   | −14.5                  | −1.58                                             | −1.84                                       |
|                                 | B3LYP      | 29.1                                                | 76.0                     | −3.60                   | −14.1                  | −1.56                                             | −1.80                                       |
|                                 | PBE        | 27.0                                                | 71.2                     | −3.38                   | −13.3                  | −1.45                                             | −1.69                                       |
|                                 | LDA        | 26.5                                                | 69.7                     | −3.31                   | −13.0                  | −1.42                                             | −1.65                                       |
| RaOCH <sub>3</sub> <sup>+</sup> | HF         | 40.0                                                | 106                      | −5.01                   | −19.7                  | −2.11                                             | −2.50                                       |
|                                 | BHandH     | 34.9                                                | 93.5                     | −4.45                   | −17.5                  | −1.88                                             | −2.23                                       |
|                                 | PBE0       | 32.8                                                | 88.1                     | −4.20                   | −16.5                  | −1.76                                             | −2.11                                       |
|                                 | B3LYP      | 32.3                                                | 87.4                     | −4.17                   | −16.4                  | −1.77                                             | −2.10                                       |
|                                 | PBE        | 30.1                                                | 81.7                     | −3.90                   | −15.3                  | −1.64                                             | −1.97                                       |
|                                 | LDA        | 29.3                                                | 79.7                     | −3.81                   | −15.0                  | −1.61                                             | −1.93                                       |
| RaCH <sub>3</sub> <sup>+</sup>  | HF         | 45.4                                                | 113                      | −5.25                   | −20.6                  | −2.17                                             | −2.54                                       |
|                                 | BHandH     | 39.0                                                | 98.5                     | −4.62                   | −18.1                  | −1.91                                             | −2.24                                       |
|                                 | PBE0       | 35.7                                                | 90.9                     | −4.27                   | −16.7                  | −1.77                                             | −2.08                                       |
|                                 | B3LYP      | 34.5                                                | 88.5                     | −4.17                   | −16.3                  | −1.74                                             | −2.03                                       |
|                                 | PBE        | 31.1                                                | 80.9                     | −3.82                   | −15.0                  | −1.60                                             | −1.87                                       |
|                                 | LDA        | 30.7                                                | 80.1                     | −3.79                   | −14.9                  | −1.59                                             | −1.85                                       |
| RaCN <sup>+</sup>               | HF         | 36.1                                                | 95.0                     | −4.50                   | −17.7                  | −2.01                                             | −2.26                                       |
|                                 | BHandH     | 32.5                                                | 86.4                     | −4.10                   | −16.1                  | −1.82                                             | −2.06                                       |
|                                 | PBE0       | 31.2                                                | 82.8                     | −3.93                   | −15.4                  | −1.73                                             | −1.97                                       |
|                                 | B3LYP      | 30.6                                                | 81.5                     | −3.87                   | −15.2                  | −1.73                                             | −1.95                                       |
|                                 | PBE        | 28.9                                                | 77.2                     | −3.67                   | −14.4                  | −1.62                                             | −1.85                                       |
|                                 | LDA        | 28.4                                                | 76.0                     | −3.62                   | −14.2                  | −1.60                                             | −1.82                                       |
| RaNC <sup>+</sup>               | HF         | 35.6                                                | 94.9                     | −4.51                   | −17.7                  | −2.01                                             | −2.28                                       |
|                                 | BHandH     | 32.0                                                | 86.1                     | −4.10                   | −16.1                  | −1.82                                             | −2.08                                       |
|                                 | PBE0       | 30.3                                                | 81.5                     | −3.88                   | −15.2                  | −1.71                                             | −1.97                                       |
|                                 | B3LYP      | 30.1                                                | 81.3                     | −3.87                   | −15.2                  | −1.73                                             | −1.97                                       |
|                                 | PBE        | 28.3                                                | 76.6                     | −3.66                   | −14.4                  | −1.62                                             | −1.86                                       |
|                                 | LDA        | 27.7                                                | 75.1                     | −3.58                   | −14.1                  | −1.59                                             | −1.82                                       |

\* konstantin.gaul@chemie.uni-marburg.de

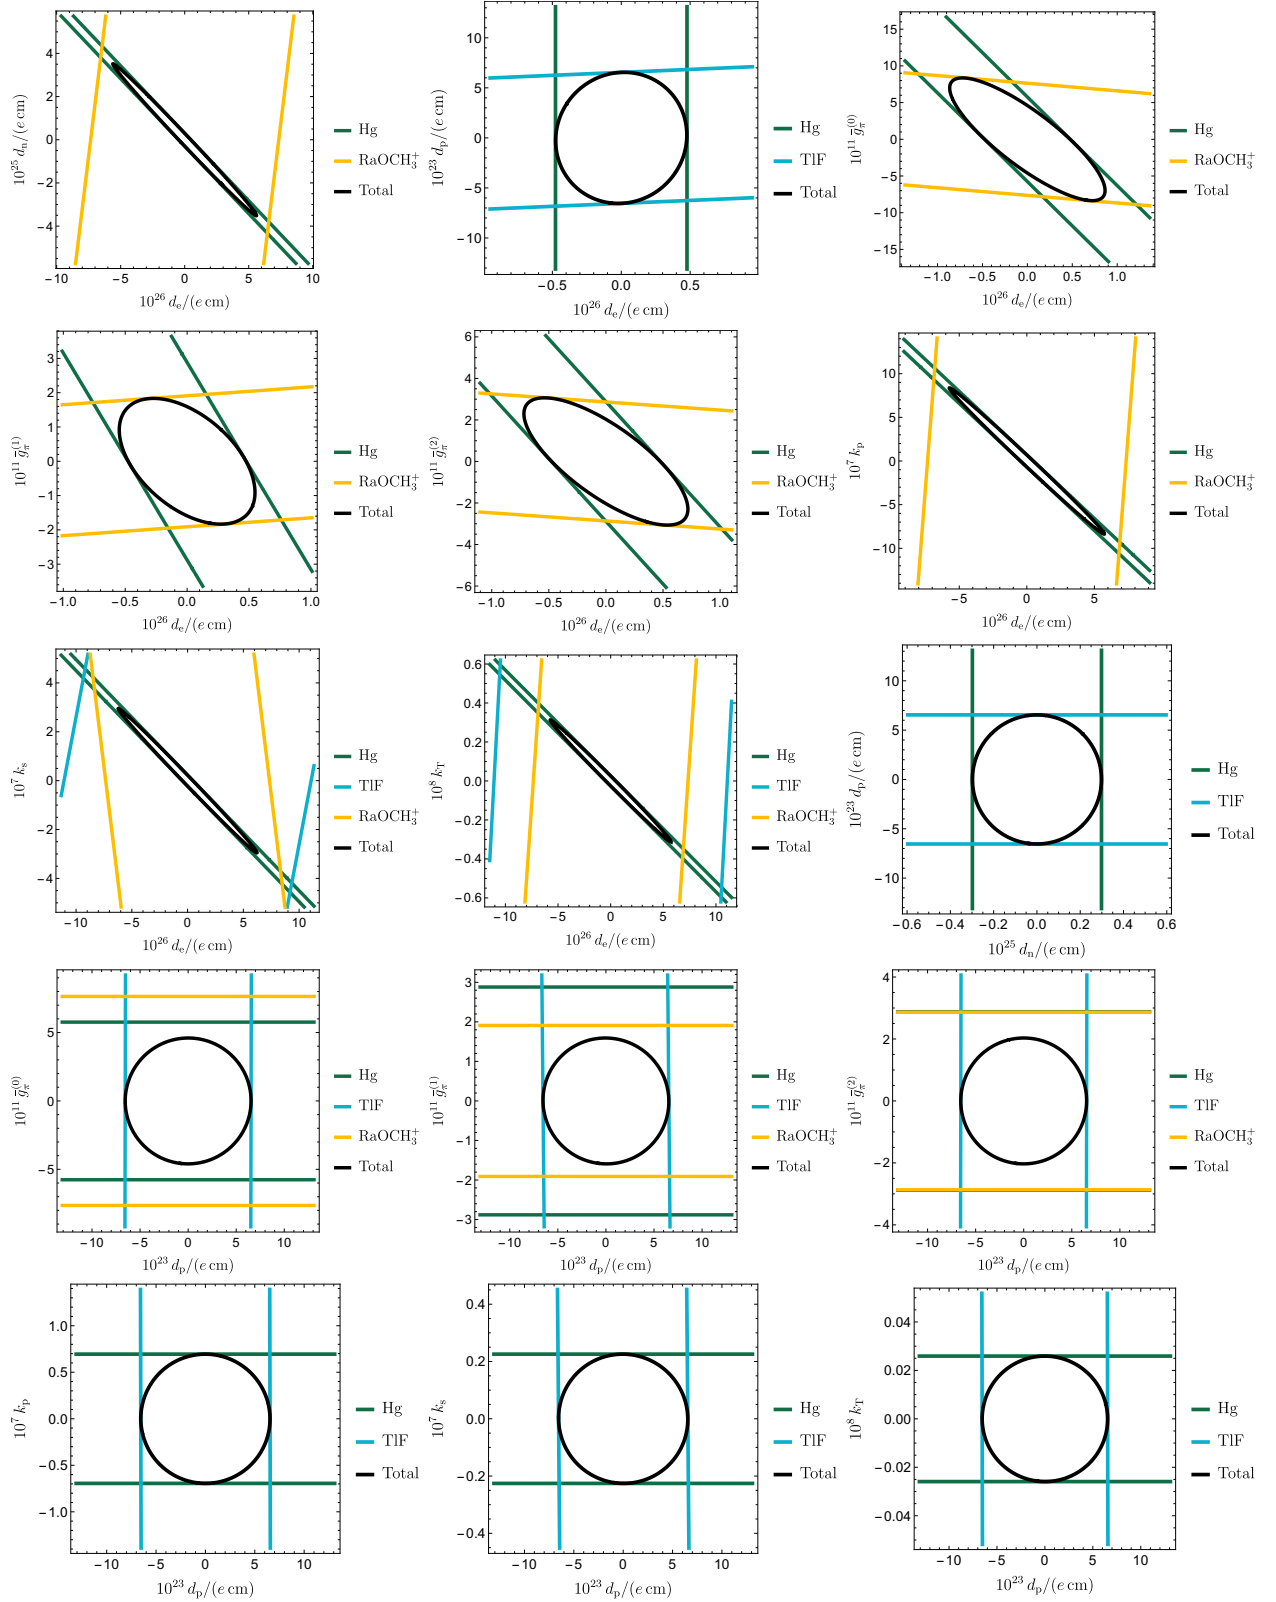

Figure 1. Restriction of two dimensional subspaces including parameters  $d_e$ ,  $d_{sr,p}$ ,  $k_s$  of the nine dimensional space of  $P, T$ -odd parameters by experiments with Hg, TlF and the proposed experiment with  $\text{RaOCH}_3^+$  excluding the pEDM. Coverage regions are computed with electronic structure parameters of  $\text{RaOCH}_3^+$  provided in this work, electronic structure parameters of TlF and Hg from Ref. [1] and nuclear structure parameters from Ref. [2]. Experimental uncertainty on the EDM of TlF  $\sigma_d = 2.9 \times 10^{-23} e\text{ cm}$  with an external electric field for polarization of strength  $\mathcal{E} = 16000 \text{ V cm}^{-1}$  is taken from Ref. [3] and on the EDM of Hg  $\sigma_d = 3.1 \times 10^{-30} e\text{ cm}$  is taken from Ref. [4]. The expected uncertainty of an experiment with a single  $\text{RaOCH}_3^+$  molecule  $\delta\nu \approx 6.5 \times 10^{-5} \text{ Hz}$  is used as proposed in Ref. [5]. All bounds are computed with Gaussian probability distributions of 95% CL as described in Ref. [1].

- 
- [1] K. Gaul and R. Berger, arXiv **hep-ph**, 2312.08858 (2023).
  - [2] T. E. Chupp, P. Fierlinger, M. J. Ramsey-Musolf, and J. T. Singh, *Rev. Mod. Phys.* **91**, 015001 (2019).
  - [3] D. Cho, K. Sangster, and E. A. Hinds, *Phys. Rev. A* **44**, 2783 (1991).
  - [4] B. Graner, Y. Chen, E. G. Lindahl, and B. R. Heckel, *Phys. Rev. Lett.* **116**, 161601 (2016).
  - [5] P. Yu and N. R. Hutzler, *Phys. Rev. Lett.* **126**, 023003 (2021).
